# Supplementary material for: A Fixed-Point Approach for Causal Generative Modeling
Source: arXiv:2404.06969 source file (2024-12-13)
Supplement: Supplementary file 1 [file appendix_notations.tex]

\section{Notations.}
